# Supplementary material for: Object Graph Programming
Source: arXiv:2402.02642 source file (2024-02-04)
Supplement: Supplementary file 1 [file supplementary.tex]

\section{Checking Class Invariants}
\begin{figure}[t]%
	\subcaptionbox{%
	  \FigKoratBTreeDefCaption%
      \hspace*{6cm}
		\label{figure:korat_example_btree_def}} {%
		\hspace*{-3cm}%
		\lstinputlisting[language=small-java-pretty]{code/code-bTree-definitions.java}%
	}\\
	\subcaptionbox{%
		\FigKoratImperativeCaption%
		\label{figure:korat_example_imperative}}{%  
		\hspace*{-1mm}%
		\lstinputlisting[language=small-java-pretty]{code/code-korat-imperative-repOK.java}%
	}\\
	\subcaptionbox{%
		\FigKoratOGOCaption%
		\label{figure:korat_example_ogo}}{%
		\lstinputlisting[language=small-java-pretty]{code/code-korat-ogo-repOK.java}%
	}
	\caption{\FigKoratCaption}%
	\label{figure:korat_example}%
\end{figure}%

\Korat is a framework developed for bounded-exhaustive test input
generation. Based on a specified predicate and a bound on the inputs,
\Korat exhaustively generates all inputs for which the predicate is
satisfied. The predicate, generally referring to the class invariants
is traditionally specified using the \Code{repOK} method. We show that
\Tool can be used to significantly simplify the implementation of the
\Code{repOK} method relative to a purely imperative approach.

We use the binary tree class defined in
Figure~\ref{figure:korat_example_btree_def} as the example. Since the
binary tree is a rooted ordered tree, its class invariants under any
mutable/immutable operation enforce that (1) the tree remains acyclic,
(2) the tree is rooted or contains atmost one node without a parent,
(3) every node in the tree has atmost 2 children and, (4) the tree is
ordered or all the left/right children store values smaller/larger
than the parent. We disregard the ordering class invariant in the
considered example. A purely imperative implementation for checking
these class invariants is given in
Figure~\ref{figure:korat_example_imperative}. A worklist algorithm is
used to traverse the tree and identify cycles thus checking the
acyclicity invariant. If no cycles are found then the number of
visited nodes must be consistent with the size of the tree to ensure
that every node in the tree is reachable from the root node which
checks if the tree is rooted. The invariant of every node having
atmost 2 children is implicitly satisified by the \Code{Node} class
definition. In contrast, the \Tool implementation is given in
Figure~\ref{figure:korat_example_ogo}. The first \Code{MATCH} clause
matches all nodes (constrained to \Code{Node} instances) reachable
from the root node under transitive closure through reference fields
\Code{left} or \Code{right}. The next clause, \Code{OPTIONAL}
\Code{MATCH} matches all nodes (constrained to \Code{Node} instances)
that are reachable from itself under transitive closure through
reference fields \Code{left} or \Code{right}. This pattern must have
atleast one relationship or in other words a node cannot
self-reference itself without a relationship. Thus, this clause
matches both, directed and undirected cycles in the tree. Finally, the
boolean expression in the \Code{RETURN} clause is used to check the
invariants. The first equality comparison expression checks if the
number of nodes reachable from root is consistent with the size of the
tree (tree is rooted). The second equality comparison expression
checks if the number of nodes reachable from themselves is 0 (tree is
acyclic).

The \Tool implementation is less verbose and more precise in terms of
its intent relative to the purely imperative implementation.
