# Supplementary material for: Object Graph Programming
Source: arXiv:2402.02642 source file (2024-02-04)
Supplement: Supplementary file 2 [file appendix.tex]

\appendix

\section{\Tool in Object Serialization}

Serialization refers to the conversion of the state of an object into
a byte stream. This allows the state of the object to be saved or
communicated across a network. Serialization is implemented using
\Java \textit{Reflections}. When an object is serialized, firstly, a
detailed description (name, type and value) of its primitive fields
obtained through \textit{Reflection} is written to a byte
stream. Second, its reference fields are accessed recursively and the
step outlined earlier is repeated. Since serialization essentially
involves visiting every object reachable from a specified root object
and logging their primitive field descriptions, \Tool is well suited
for implementing it. Fig.~\ref{listing:Serialization-field-value}
-~\ref{listing:Serialization-object-value} compares
\textit{Reflection} vs. \Tool approach.
